# Supplementary material for: Speed Scaling with Tandem Servers
Source: arXiv:1907.04498 source file (2019-07-10)
Supplement: Supplementary file 1 [file Appendix2.tex]

\section{Proof of Lemma \ref{lem:jumpSP}}
\begin{enumerate}
\item Before any job arrives and after all jobs are finished, $\Phi(t)= 0$.  With the above speed scaling algorithm, this is clearly true.
\item Bounding the increase in $\Phi(t)$ on any jump discontinuity. 
There are possible $3$ ways that give rise to a discontinuity because of the algorithm. 
\begin{enumerate} 
\item Job arriving at server $1,1$ at time $t$. If server $1,1$ is already active at time $t$, then there is no change to the $\Phi(t)$ since $A(t)$ remains unchanged, and both $n^{11}(t,q)$, and $n^{11}_o(t,q)$ increase by $1$ for all $q\in [0,1]$. 
In case, server $1$ is inactive just before time $t$, then as described in Remark \ref{rem:jumpSP}, the size of the outstanding job on active server $2,1$ is made $q_{21}=1$. This can result in increase in the potential function $\Phi(t)$ which we upper bound as follows. 
Note that in this sub-case $A(t)$ increases by $1$, since server $1$ has become active, while no other inactive server has become active or any active server has become inactive. The only potential function that changes at time $t^+$ because of increasing the job size is $\Phi_{21}(t)$, which is  
\begin{align*}
\Phi_{21}(t^+) =   c_{21} \int_{0}^1 f\left(\frac{d^{21}(t^+,q)}{A(t)+1}\right) dq,
\end{align*}
where 
\begin{align*} d^{21}(t^+,q)& \le \max\left\{0,  \left((n^{11}(t) - n^{11}_o(t))  + \max\left\{n^{21}(t,q)+1 - n^{21}_o(t,q)\right\}\right) \right\}.
\end{align*}
since $n^{11}(t^+)-n^{11}_o(t^+)\le 0$ as $n^{11}(t)=0$, and $n^{21}(t^+,q)\le n^{21}(t,q)+1$ because of increasing the size of job in active server $21$. Thus, $d^{21}(t^+,q) \le A(t)+1$ for all $j$ since $n^k(t)\le 1$ for all servers $k\ge 2$, and we have $f\left(\frac{d^{21}(t^+,q)}{A(t)+1}\right)\le f(1)$. This implies that  
\begin{align*}
\Phi_{21}(t^+) \le   c_{21} f(1), 
\end{align*}
and
\begin{align}\label{eq:jump1sp}
\Phi(t^+) \le   c_{21} f(1).
\end{align}
Thus, the jump $\Phi(t^+) - \Phi(t)\le c_{21} f(1)$ in the potential function is bounded even when we are increasing the job sizes of existing jobs in active servers on arrival of a new job in server $1$ at the time when server $1$ is inactive.

\item Job transitioning from server $1,1$ to $2,j$ $j\ge 2$  at time $t^+$. 
Recall that $n^{2,1}$ is either $0$ or $1$. If it is $0$, then a job moving from server $1,1$ to $2,j$ $j\ge 2$ either does not change $A(t)$ (remains $1$ if $n^{2,1}(t) > 1$) or server $1$ itself become inactive. In the first case, $d_{11}(t,q)$ changes only for $q=0$, keeping $\Phi_{11}(t)$ unchanged, while $d^{2j}(t,q)$ increases by $1$ for $q\in[0,1]$, and thus \begin{equation}\label{eq:jump2sp}
\Phi_{2j}(t^+)\le c_{2j}f(1).
\end{equation} Moreover, if $n^{2,1}(t) =1$, then a job from server $1,1$ moves to server $2,j$ for $j\ge 2$, if  $n^{2,1}(t^+) = 0$ since the movement of jobs from server $1,1$ and $2,1$ is synchronized because of Remark \ref{rem:jumpSP}. [XXX Write better]

\item Job transitioning from server $1,1$ to $2,1$ at time $t^+$. With the proposed algorithm in light of  Remark \ref{rem:jumpSP}, job transitions between servers $1,1$ and $2,1$ are synchronized, i.e., if job is moving from server $1,1$ to $2,1$, then if there was a job on server $2,1$ then that job is leaving the system at time $t$. Thus, either $A(t)$ remains same if $n^{11}(t) > 1$ or $A(t^+) = A(t)-1$ if $n^{11}(t) \le 1$. In first case, $d^{ij}$ changes only for $q=0$ and keeps the potential function $\Phi(t)$ unchanged. In second case, $\Phi_{11}(t^+)=0$ since $n^{11}(t^+) =0$, and 
we can upper bound the change in the potential function $\Phi_{21}(t)$ as follows. Since each active server has at most one unfinished job, and $n^{11}(t) \le 1$, $d^{21}(t^+,q) \le A(t)-1$ and hence
\begin{align}\label{eq:jump2sp}
\Phi_{21}(t^+) & =   c_{21} \int_{0}^1 f\left(\frac{d^{21}(t^+,q)}{A(t)-1}\right) dq \le c_{21} \int_0^1 f(1) dq \le c_{21}f(1).
\end{align}

Finally, we consider the case when a job moves from server $1,1$ to $2,j$ with the $\opt$ or a job departs the system from any server of layer $2$ with the $\opt$. 
In the first case, $A(t)$ does not change, and $d^{ij}(t,q)$ only changes for $q=0$ thus, does not affect the integral in $\Phi_{ij}(t)$, keeping it unchanged. When a job departs from the system $d^{2j}(t,q)$ only changes for $q=0$, and $\Phi_{ij}(t)$ remains unchanged.
\end{enumerate}
\end{enumerate}
Since there are at most $n$ jobs, there are at most $n$ points of discontinuities. From \eqref{eq:jump1sp} and \eqref{eq:jump2sp}, we know that the cumulative increase in $\Phi$ is at most $(c_{21} + c_{2j})f(1)$ for some $j\ge 2$, for each such discontinuity.  Result follows by choosing $c_{ij} = c$ for all servers $i,j$ in \eqref{defn:phi}.

\section{Proof of Lemma \ref{lem:driftSP}}
Let $q^{ij}_a$ and $q^{ij}_o$ be the remaining size of the job that server $i,j$ is executing with the algorithm and the $\opt$ respectively. Then from the definition of $\Phi_{ij}(t)$ \eqref{defn:phiSP},  similar to \eqref{eq:dummy3} and \eqref{eq:dummy4}, for servers $1,1$ and $2,1$, if $q^{i1}_a < q^{i1}_o$ we get that 
\begin{align}\label{eq:dummy3sp}
d\Phi_{i1}(t)/dt & = c_{i1} \Delta \left( \frac{\sum_{k=1}^{i-1} (n^{i1}(t) - n^{i1}_o(t)) + n^{i1} -  n^{i1}_o}{A(t)}\right)(-s_{i1} + s_{i1}^o),
\end{align}
and
\begin{align}\label{eq:dummy4sp}
d\Phi_{i1}(t)/dt & = c_{i1}\Delta \left( \frac{\sum_{k=1}^{i-1} (n^{i1}(t) - n^{i1}_o(t)) + n^{i1} -  n^{i1}_o+1}{A(t)}\right)(-s_{i1} + s_{i1}^o),
\end{align}
if $q^{i1}_a\ge q^{i1}_o$. 
Similarly, for servers $2,j$ for $j\ge 2$,   
if $q^{2j}_a < q^{2j}_o$ we get that 
\begin{align}\label{eq:dummy5sp}
d\Phi_{2j}(t)/dt & = c_{2j} \Delta \left(  n^{2j} -  n^{2j}_o\right)(-s_{2j} + s_{2j}^o),
\end{align}
and
\begin{align}\label{eq:dummy6sp}
d\Phi_{2j}(t)/dt & = c_{2j}\Delta \left(  n^{2j} -  n^{2j}_o+1\right)(-s_{2j} + s_{2j}^o),
\end{align}
if $q^{2j}_a\ge q^{2j}_o$. 
Now, we apply technical Lemma \ref{lem:bansal}, to bound the RHS of \eqref{eq:dummy4sp} with $\beta = \left( \frac{\sum_{k=1}^{i-1} (n^{i1}(t) - n^{i1}_o(t)) + n^{i1} -  n^{i1}_o+1}{A(t)}\right)$ and noting the fact that $s_{i1} \ge P^{-1}(\beta)$ \eqref{eq:speeddefSP} gives that 
$d\Phi_{i1}/dt\le  c_{i1} P(s_{i1}^o) - c_{i1} \frac{n^{11}(t) + i-1}{A(t)} + c_{i1} \frac{n^{11}_o(t) + \sum_{i=1}^{2}\b1^{i1}_o(t) n^{i1}_o(t)}{A(t)}$.
Similarly, if we choose $\beta =  n^{2j} -  n^{2j}_o$ for \eqref{eq:dummy5sp} and apply  Lemma \ref{lem:bansal}, and use the fact that $s_{2j} = P^{-1}(2) \ge P^{-1}(n^{2j})$ since $n^{2j}\le 1$, we get 
$$d\Phi_{2j}/dt\le c_{2j} P(s_{2j}^o) - c_{2j} n^{2j}(t) + c_{2j}n^{2j}_o(t),$$
as required.
